# Supplementary material for: A Primal-Dual Framework for Symmetric Cone Programming
Source: arXiv:2405.09157 source file (2024-05-15)
Supplement: Supplementary file 1 [file appendix.tex]

\section{Omitted proofs}

\subsection{Proof of Theorem~\ref{thm:ses}}
\label{sec:ses_proof}

\subsection{Proof of Theorem~\ref{thm:svm}}\label{sec:svm_proof}
